# Supplementary material for: A Case for Superconducting Accelerators
Source: arXiv:1902.04641 source file (2019-02-14)
Supplement: Supplementary file 1 [file Appendix.tex]

\newpage
%%% ISCA template does not allow appendix after references -- Appendix needs to be a section
\section{Appendix}
\subsection{Superconducting Logic Using RQL}
\label{rql_background}
Since their introduction in the late 1960's, Josephson Junction based digital circuits have been studied as suitable devices to enable faster digital information processing. Until the late 1990's, several circuits were demonstrated with extremely high operational frequencies. However, these early superconducting circuits used  DC biased JJs with bias resistors to distribute power on a common voltage rail. These bias resistors contributed to sizeable static power dissipation limiting the scalability of resistor biased SFQ (RSFQ) circuits.  Recently proposed, Reciprocal Quantum Logic (RQL) overcomes the drawback of static power dissipation of RSFQ~\cite{herr2011ultra}. It uses AC power lines and inductive coupling to distribute power and clock to the devices in the circuit. It also uses lower device counts per gate as compared to RSFQ. These factors  enable negligible static power dissipation and higher logic-gate density in RQL circuits. The AC power line serves as a stable reference clock signal and prevents accumulation of clock jitter and noticeable timing variations. 
%% Describe RQL briefly

\subsection{Operation of RQL gates}

In RQL, a digital ``1" is encoded as a pair of SFQ pulses of opposite polarity and a ``0" is encoded as the absence of SFQ pulses as shown in Figure ~\ref{fig:rql_basics}(a). The logical behavior of the gates is based on the reciprocal data encoding. For a digital ``1", operations with the positive SFQ pulse involve storage and routing of SFQ data. When only the positive pulses are considered, the gates act like state machines, as the input changes, the internal flux state of the inductive loops changes as well. The negative pulse resets the internal state of the RQL cells every clock cycle to the initial state and produces combinational logic behavior. The erasing operation facilitated by the negative pulse simplifies the logic design, to the extent that some gates can comprise of as low as only two active devices with biasing inductors.

\begin{figure}[!htb]
 \vspace{0.1in}
    \includegraphics[width=1.0\columnwidth]{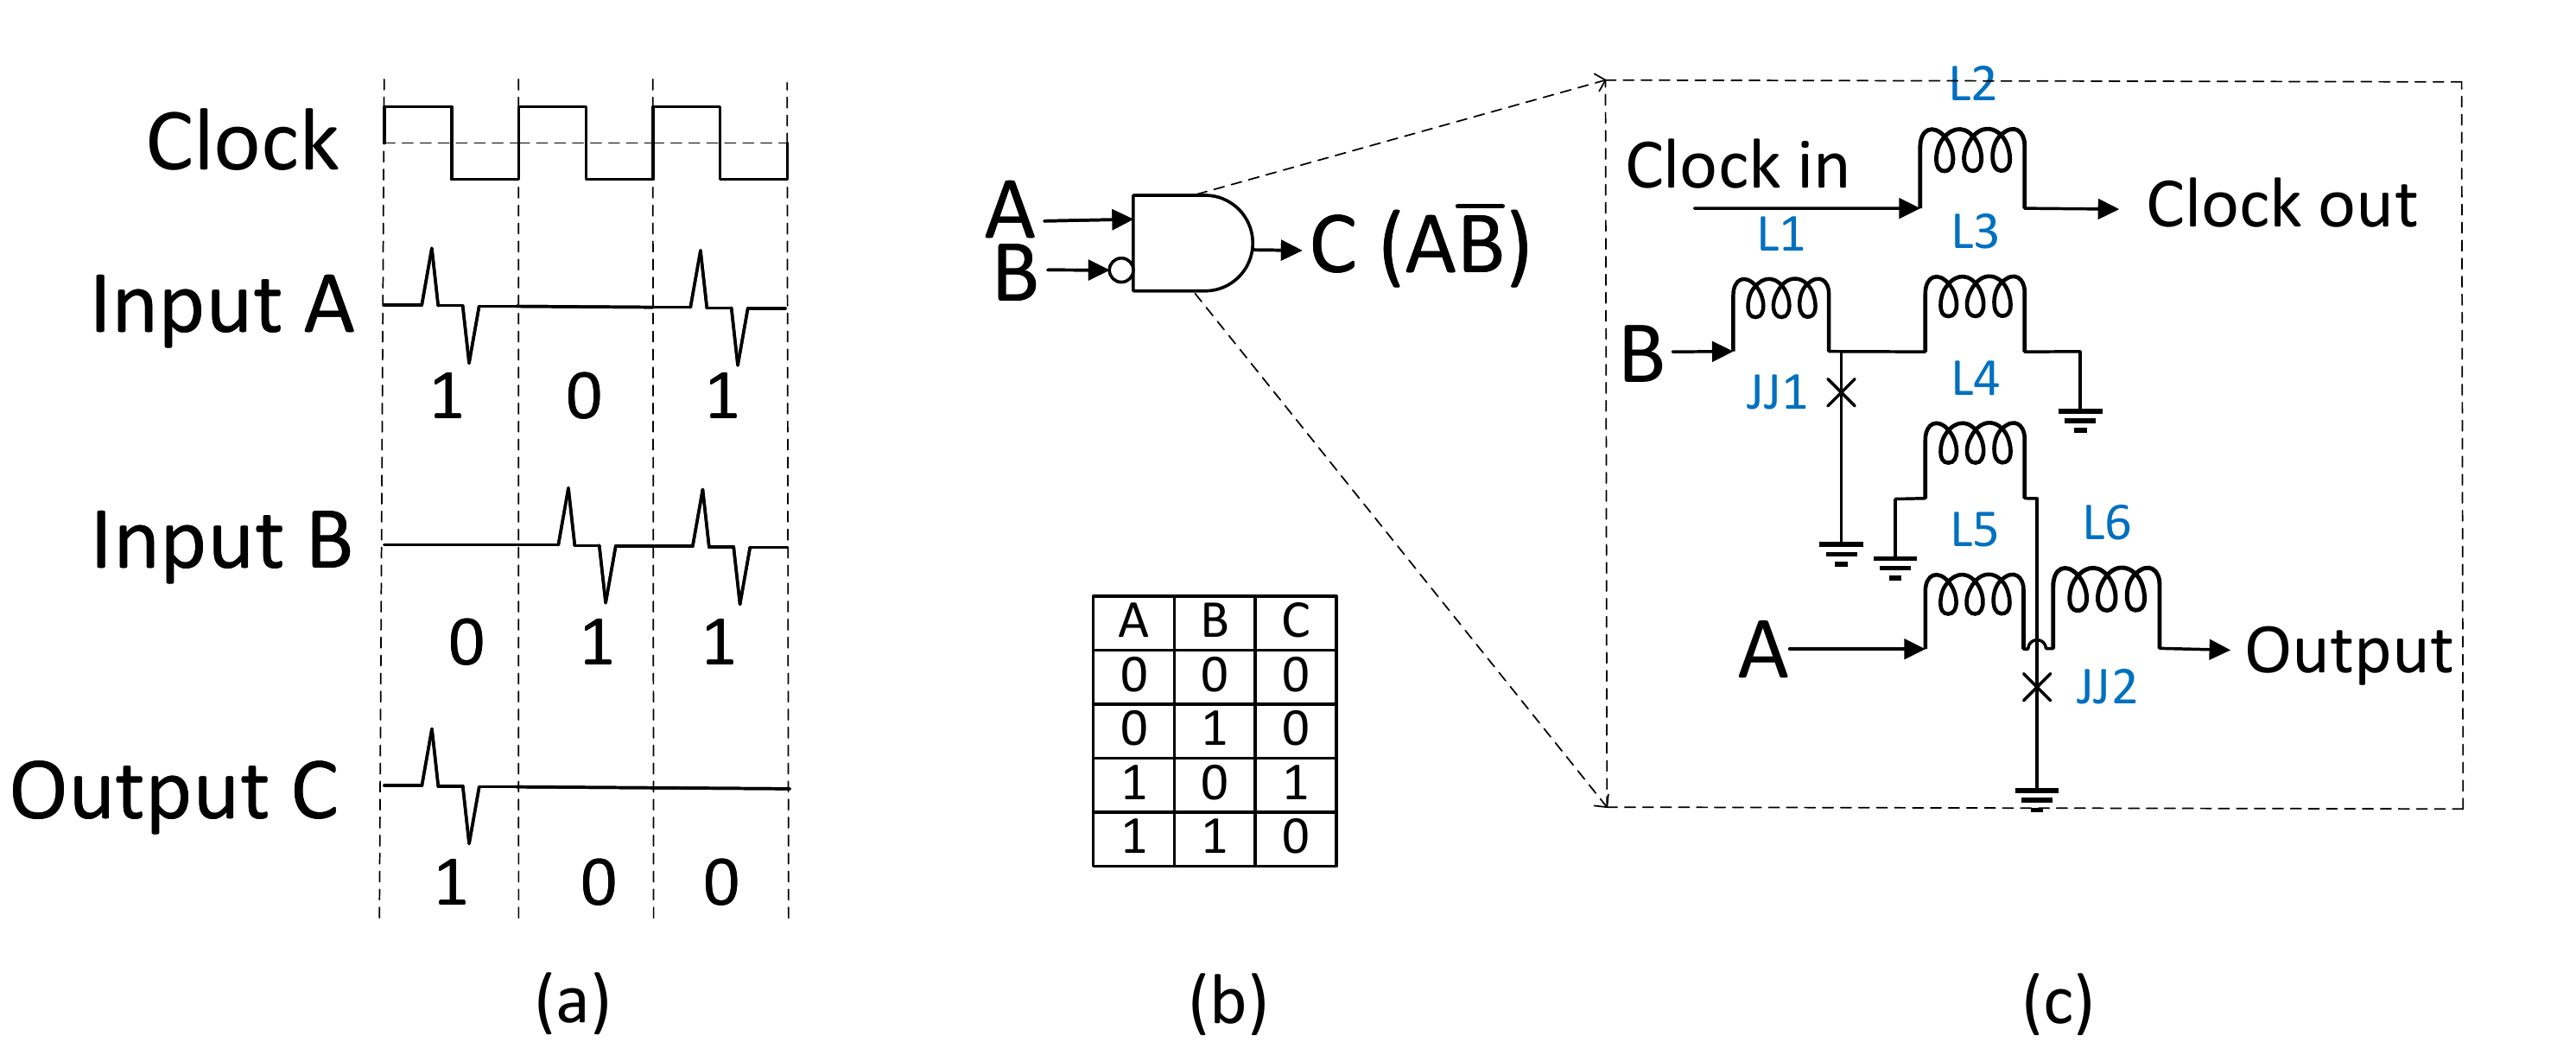}
 %    \vspace{-0.25in}
    \caption{a) Data encoding in RQL and A-AND-NOT-B logical operation (b)Gate symbol (c) Circuit schematic}
    \label{fig:rql_basics}
 %    \vspace{-0.15in}
\end{figure}

%% Describe the RQL logic family
%The RQL family consists of two universal gates, the AND-OR gate and the A-AND-NOT-B gate that enables the design of other gates and complex circuits~\cite{herr2011ultra,oberg2011superconducting}. 
Figure ~\ref{fig:rql_basics}(b) and ~\ref{fig:rql_basics}(c) shows the schematic of an A-AND-NOT-B gate~\cite{oberg2011superconducting}. This gate allows any pulse incoming at A to pass through to the output as long as a pulse has not arrived at B earlier. The two Josephson junctions JJ1 and JJ2 are connected to each other through a high efficiency transformer. This enables the junctions to be negatively coupled to each other. When a positive current flows through one of the junctions, it induces a negative current in the other junction. 
As a result, during an operation when a pulse arrives at input B, it switches JJ1 and prevents JJ2 from switching by inducing a negative current through it. Post this, when a pulse arrives at the input A, it cannot propagate to the output. Alternately, when there is no pulse at input B, JJ2 switches and generates an output. For this particular gate to function as intended, strict timing requirements on the arrival of a pulse at the B input port must be adhered to. For operation of other RQL universal gates, one may refer to~\cite{oberg2011superconducting}.
%% Circuits demonstrated
%Since its introduction in 2011, RQL circuits with 72800 JJs were demonstrated. Demonstrated circuits includes shift registers and other arithmetic circuits~\cite{herr20138, herr2015reproducible}. Furthermore, design and resources were estimated for some key components of a processor such as 32-bit and 64-bit integer and floating-point arithmetic and logical units, register file, and limited form of on-chip memory~\cite{dorojevets2015towards,dorojevets2015fast}.

\subsection{Delay Line Memory}

Delay line memory in a form of memory used in earliest computers during the 1960s~\cite{eckert1953memory,auerbach1949mercury}. Unlike modern day random access memories, a delay line memory is based on sequential access and requires to be refreshed from time to time. Such memories rely on transmitting information through a circuitry that adds delay and the re-routing the end of the delay path to the input end such that the information can be transmitted continuously through the closed loop as shown in Figure~\ref{fig:dlm}. Data is retained in the memory as long as power is on. The information in such a memory is stored in the form of electrical and acoustical impulses that keeps circulating in a medium capable of transmitting acoustic waves. Mercury served as the medium for the earliest delay line memories. The capacity of such a memory depends on the number of pulses it can store.   
\begin{figure}[!htb]
 \vspace{0.1in}
 \centering
    \includegraphics[width=0.70\columnwidth]{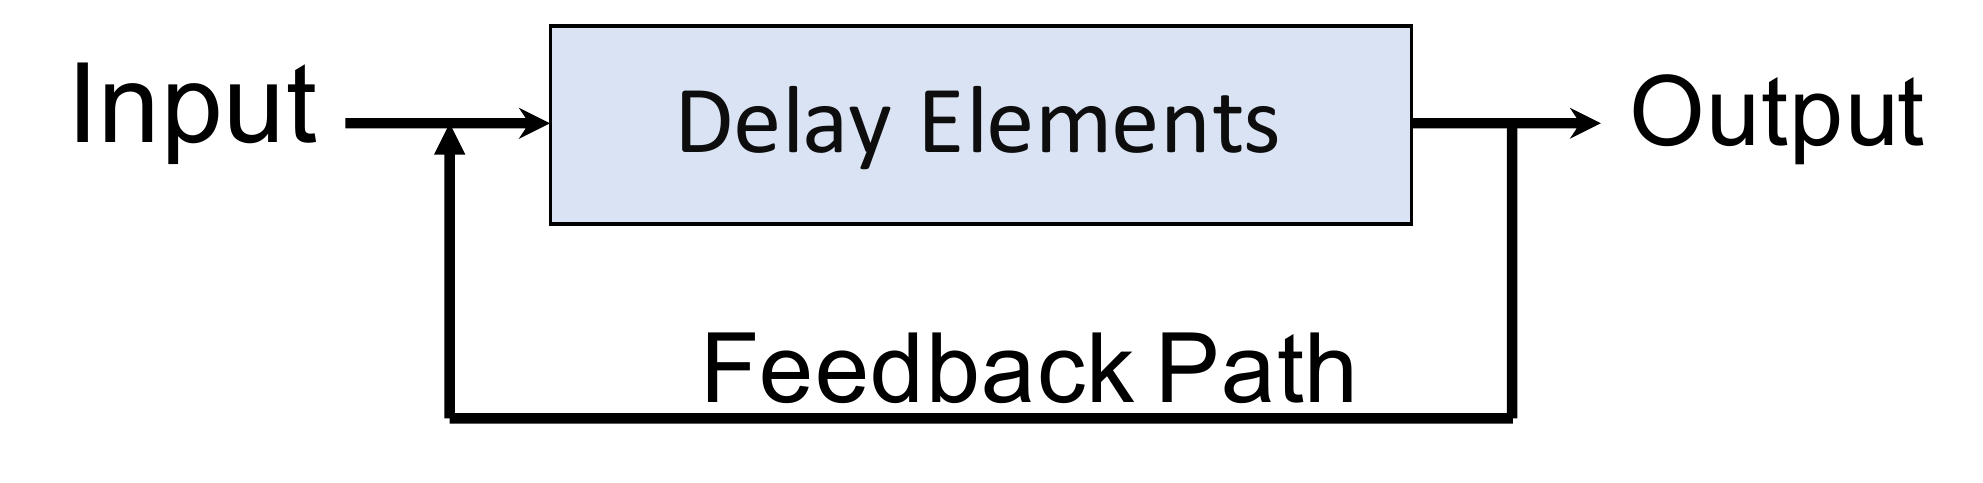}
 %    \vspace{-0.25in}
    \caption{Delay Line Memory}
    \label{fig:dlm}
 %    \vspace{-0.15in}
\end{figure}
